# Supplementary material for: Mean-Field Density Matrix Decompositions
Source: arXiv:2009.10837 ancillary file (2020-12-03)
Supplement: Supplementary file 1 [file si.pdf]

# Supporting Information:
# Mean-Field Density Matrix Decompositions


Janus J. Eriksen*

*School of Chemistry, University of Bristol, Cantock's Close, Bristol BS8 1TS, United Kingdom*

E-mail: janus.eriksen@bristol.ac.uk

# 1 Geometries

The geometry of benzene (Fig. 1 of the main work) used in our study is the MP2/6-31G* optimized structure from Ref. S1, cf. Table S1, which was also recently used in Ref. S2.

Table S1: $C_6H_6$ (in Å).

| Atom | $x$ | $y$ | $z$ |
|---|---|---|---|
| C | 0.000000 | 1.396792 | 0.000000 |
| C | 0.000000 | −1.396792 | 0.000000 |
| C | 1.209657 | 0.698396 | 0.000000 |
| C | −1.209657 | −0.698396 | 0.000000 |
| C | −1.209657 | 0.698396 | 0.000000 |
| C | 1.209657 | −0.698396 | 0.000000 |
| H | 0.000000 | 2.484212 | 0.000000 |
| H | 2.151390 | 1.242106 | 0.000000 |
| H | −2.151390 | −1.242106 | 0.000000 |
| H | −2.151390 | 1.242106 | 0.000000 |
| H | 2.151390 | −1.242106 | 0.000000 |
| H | 0.000000 | −2.484212 | 0.000000 |

The geometry of $H_2O$ (Figs. 2 and 3 of the main work) is given in Table S2.

Table S2: $H_2O$ (in Å) used in Figs. 2 and 3.

| Atom | $x$ | $y$ | $z$ |
|---|---|---|---|
| O | 0.00000000 | 0.00000000 | 0.00000000 |
| H | −0.75390364 | 0.00000000 | −0.58783729 |
| H | 0.75390364 | 0.00000000 | −0.58783729 |

The polyacetylene geometries used in Sect. 3.2 (Figs. 4 and 5) of the main work are those of Ref. S3. The alkane and water geometries of Sect. 4 (Figs. 6 through 12) of the main work have been extracted from Refs. S4 and S5.

## 2 $H_2O$ Dipole Moments

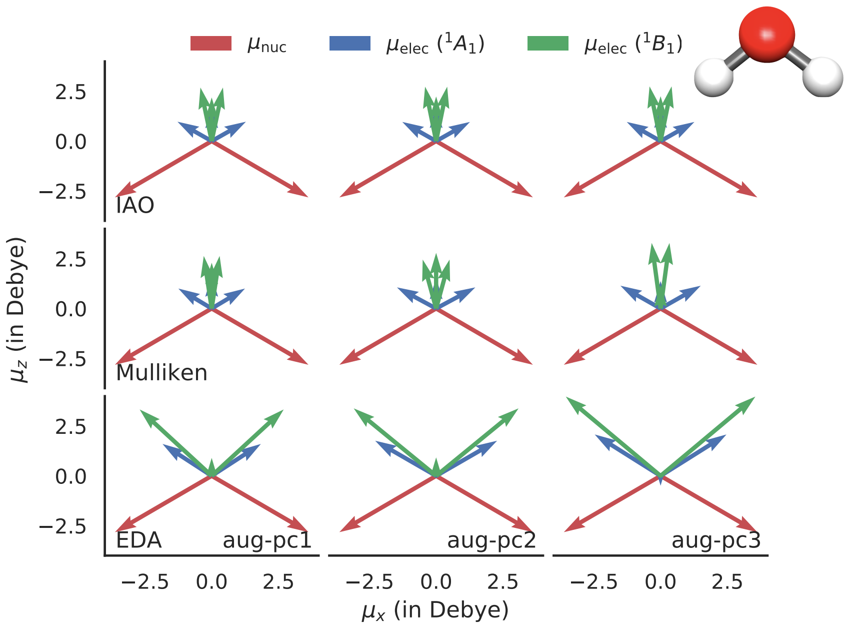


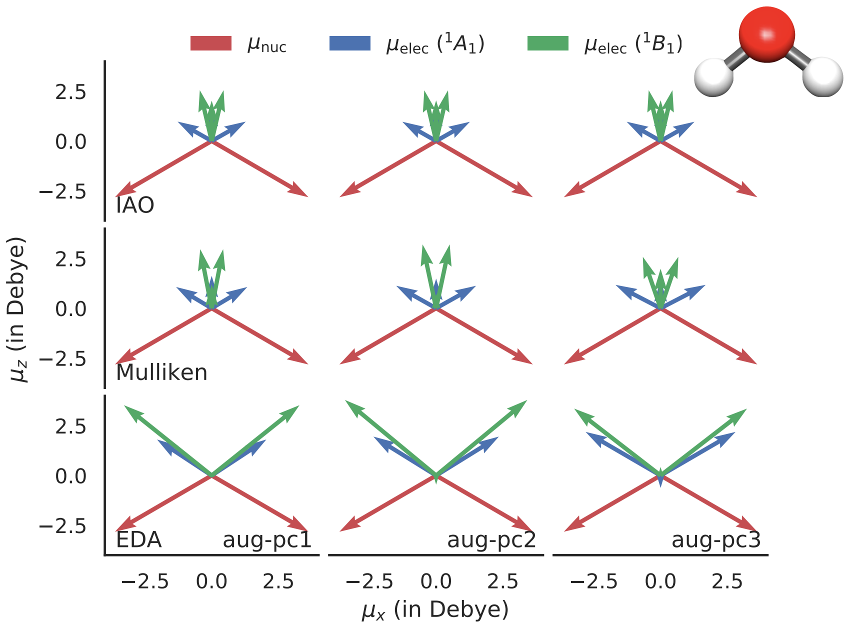


Figure S1: HF (upper panel) and M06-2X (lower panel) ground (gs) and excited (ex) state molecular dipole moments of $H_2O$ in the aug-pc$X$ basis set (in units of Debye).

# 3 $C_4H_{10}$ Thermalized Potential Energy Surface

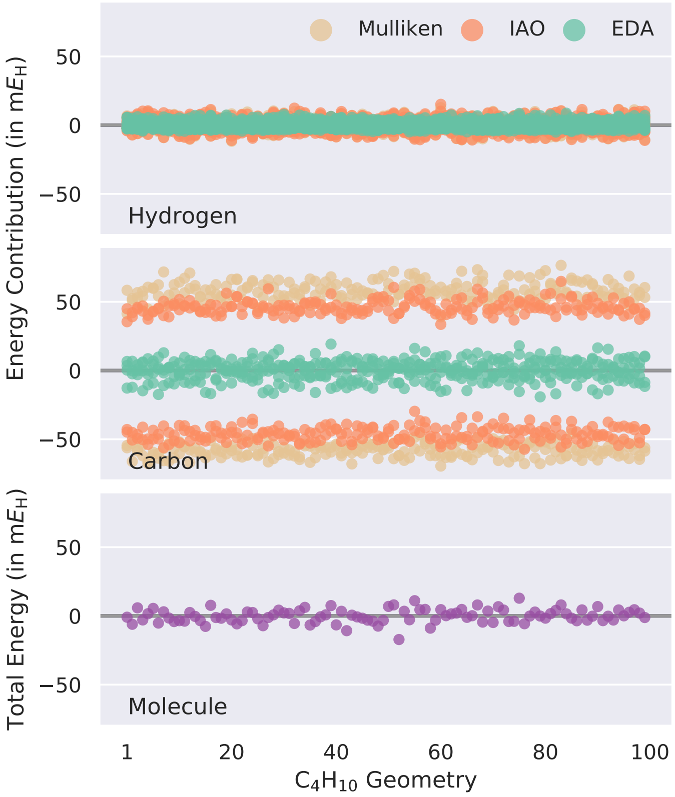


Figure S2: IBO/IAO-based B3LYP/pc-1 results for the thermalized ground state of butane, plotted like Figure 10 of the main text.

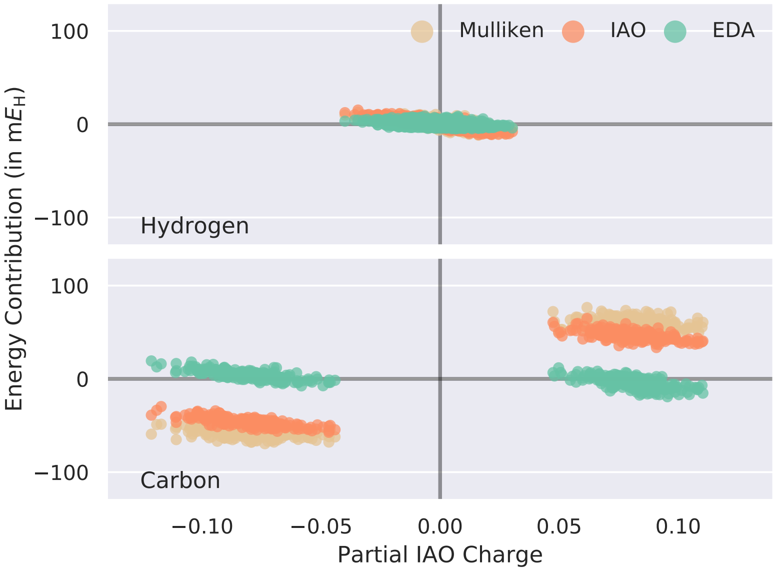


Figure S3: IBO/IAO-based B3LYP/pc-1 results for the thermalized ground state of butane, plotted like Figure 11 of the main text.

# 4 $H_2O$ Thermalized Potential Energy Surface

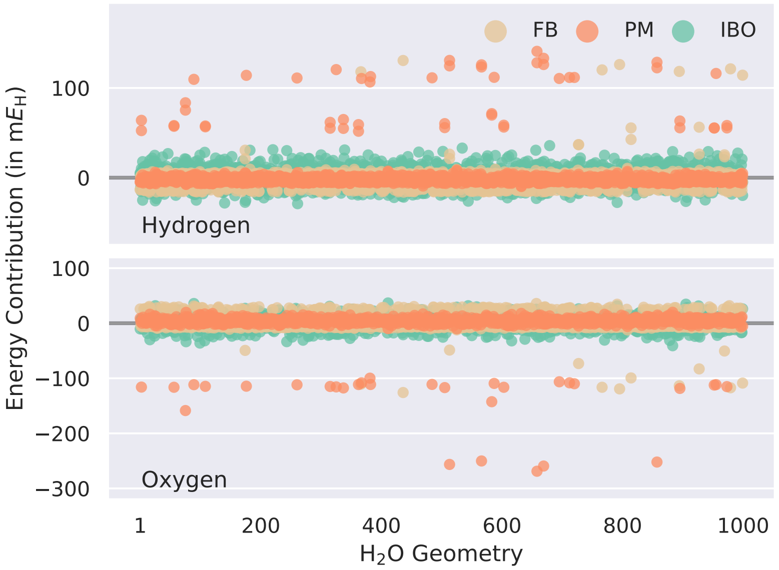


Figure S4: Same results as in Figure 10 of the main text, except obtained using different localization procedures.

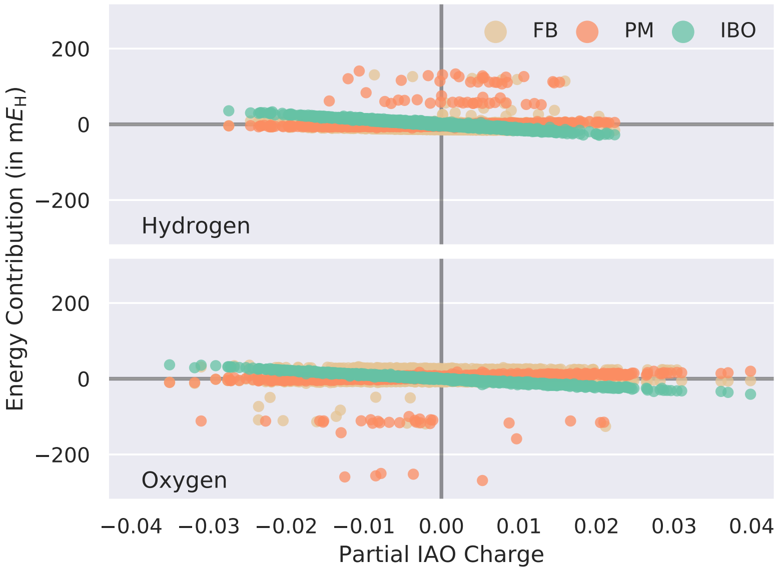


Figure S5: Same results as in Figure 11 of the main text, except obtained using different localization procedures.

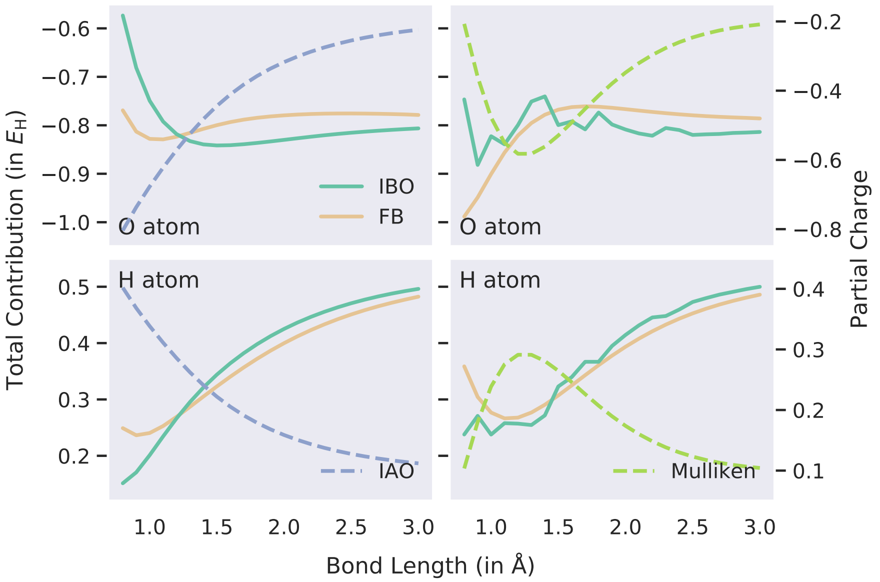


Figure S6: PES for the symmetric stretch in $H_2O$. Results are shown as contributions to atomization energies, and the corresponding partial charges, by means of which the atom-RDM1 are computed, are shown as well.

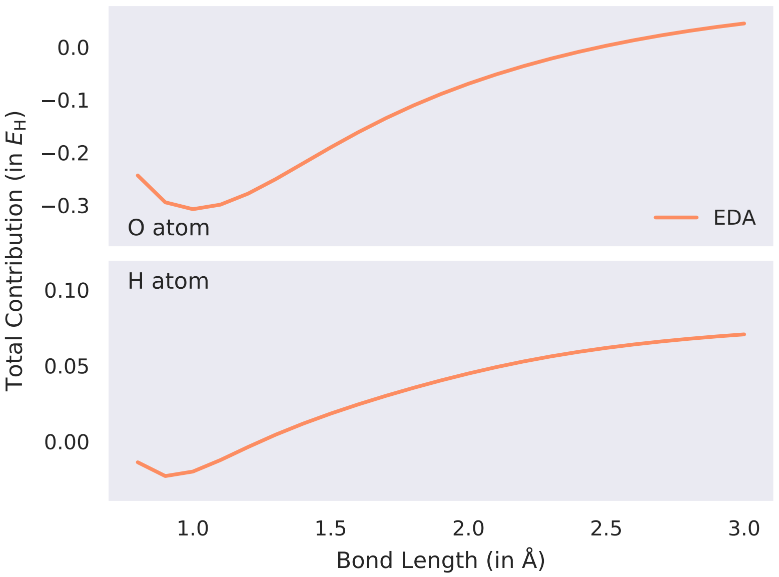


Figure S7: Same plot as in Figure S6, but computed using the EDA partitioning.

# References


(S1) Schreiber, M.; Silva-Junior, M. R.; Sauer, S. P. A.; Thiel, W. Benchmarks for Electronically Excited States: CASPT2, CC2, CCSD, and CC3. J. Chem. Phys. **2008**, 128, 134110.

(S2) Eriksen, J. J.; Anderson, T. A.; Deustua, J. E.; Ghanem, K.; Hait, D.; Hoffmann, M. R.; Lee, S.; Levine, D. S.; Magoulas, I.; Shen, J.; Tubman, N. M.; Whaley, K. B.; Xu, E.; Yao, Y.; Zhang, N.; Alavi, A.; Chan, G. K.-L.; Head-Gordon, M.; Liu, W.; Piecuch, P.; Sharma, S.; Ten-no, S. L.; Umrigar, C. J.; Gauss, J. The Ground State Electronic Energy of Benzene. J. Phys. Chem. Lett. **2020**, 11, 8922.

(S3) Sharma, P.; Bernales, V.; Knecht, S.; Truhlar, D. G.; Gagliardi, L. Density Matrix Renormalization Group Pair-Density Functional Theory (DMRG-PDFT): Singlet-Triplet Gaps in Polyacenes and Polyacetylenes. Chem. Sci. **2016**, 10, 1716.

(S4) Cheng, L.; Welborn, M.; Christensen, A. S.; Miller III, T. F. Thermalized (350K) QM7b, GDB-13, Water, and Short Alkane Quantum Chemistry Dataset Including MOB-ML Features. 2019; `https://data.caltech.edu/records/1177`, DOI: 10.22002/D1.1177.

(S5) Christensen, A. S.; von Lilienfeld, O. A. The Water40 10K Dataset. 2019; `https://figshare.com/articles/dataset/Water40_10K/8058497`, DOI: 10.6084/m9.figshare.8058497.
